# Supplementary material for: On Adversarial Robustness of Point Cloud Semantic Segmentation
Source: arXiv:2112.05871 source file (2023-04-23)
Supplement: Supplementary file 1 [file 6_supplementary.tex]

% \section{Discussion about the $c$ constant}
%\newpage
\begin{appendices}
% \zl{can you make it a new page}

%\onecolumn

\section{Supplementary Material}

\ignore{
\begin{algorithm2e}
\SetAlgoLined
\KwIn{The type of perturbation $tar=\{s| s\in \{color, coordinate\}\}$, the original point cloud $X$, the ground-truth labels $Y_{gt}$, the maximal number of iterations $Steps$, the target labels $Y_{t}$, the top $\alpha$ nearest neighbors, the learning rate $lr$, the fixed-point mask with the same shape of the point cloud $M=\{m_i\in \{ True, False \}\}$, the identity matrix $\mathbb{I}$ }

\KwOut{the adversarial perturbation $r$}
 
 $X_0 \leftarrow X, r \leftarrow X^{tar}, i \leftarrow 1, M\leftarrow \mathbb{I} $\;
 \uIf{ $tar==color$ } {
 $w=tanh^{-1}(2\cdot r-1)$\;
 }\uElseIf{ $tar==coordniate$ }{
 $w=tanh^{-1}(r)$\;
 }
 \While{$M.sum > X.point_num\cdot 1\% $ }{
  \While{$i \leq  Steps$}{
  \uIf{ $tar==color$ } {
    $X_i^{pertub}$ = $\frac{1}{2}\text{tanh(w)}+1$\;
  }\uElseIf{ $tar==coordniate$ }{
    $w=tanh^{-1}(pertub)$\;
  }

  $r$ = $X_i^{pretub} - X_{i-1}^{pertub}$\;
  $X_i$ = $X_{i-1} + r$\;

  \uIf{targeted attack}{
  $loss$ = $\mathcal{L}_{t}(X_i,Y_t)$\;
  }\uElseIf{non-targeted attack}{
  $loss$ = $\mathcal{L}_{nt}(X_i,Y_{gt})$\;
  }
  $gain_i$=$loss$\;
  $r,g$ = $Update(gain_i, lr)$\;
  \uIf{ $Converge(gain_i$)  }{
    return \;
  }
  \uElseIf{($i$ \% ($int(Steps*0.01)$) == $0$) \& ($gain_i \geq gain_{i-1}$) }{
  $r_{pertub}$ = $r_{pertub}$ + uniform noise\;
  }
  $i\leftarrow i+1$\;
 }
  $N=\argmin_{100} g\cdot r $\;
  $M = Fix(M, N)$\;
 }
 return $M$, $r_{color}$\;
 \caption{\text{The pseudo-code of coordinate-based attack.}}
\label{alg:l0 algorithm}
\end{algorithm2e}
}

\end{appendices}
